# Supplementary material for: Higgs Production and $H^0 \to c\overline{c}$ at a Future Muon-Ion Collider
Source: arXiv:2211.02615 source file (2022-11-07)
Supplement: Supplementary file 4 [file matrix.pdf]

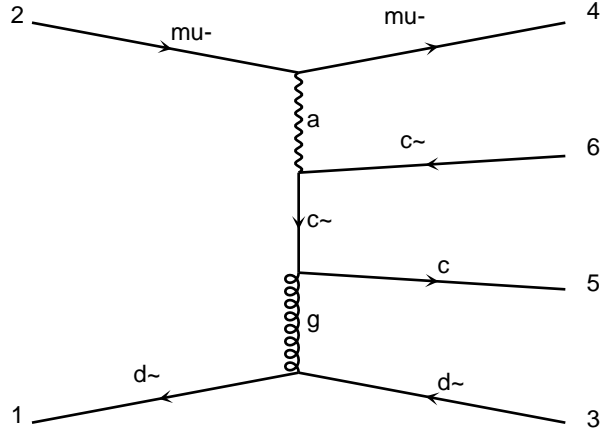

diagram 1

QCD=2, QED=2

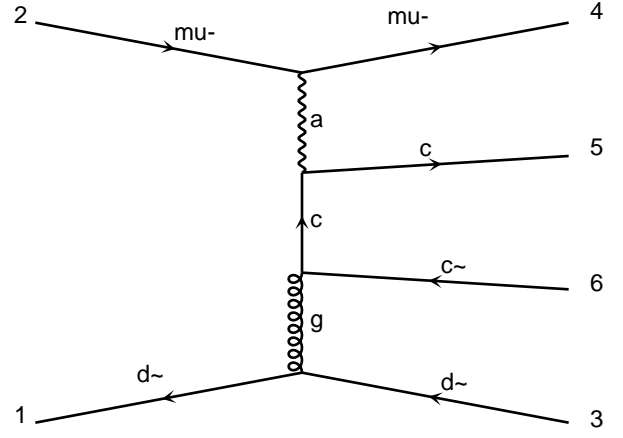

diagram 2

QCD=2, QED=2

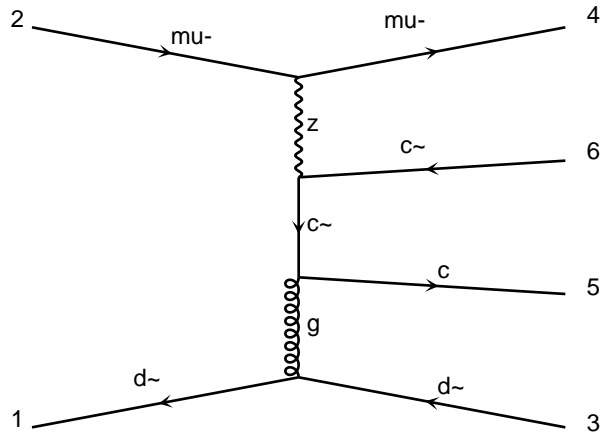

diagram 3

QCD=2, QED=2

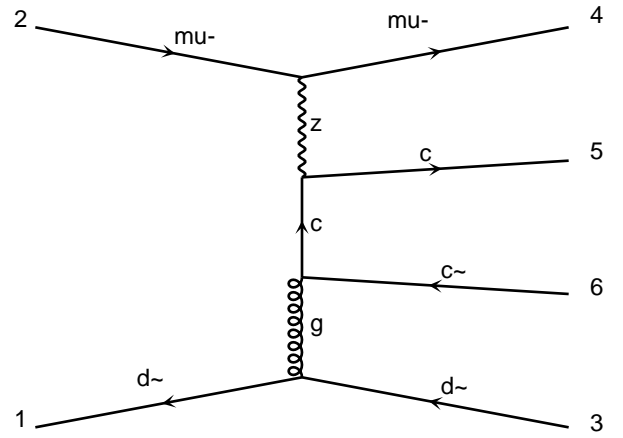

diagram 4

QCD=2, QED=2

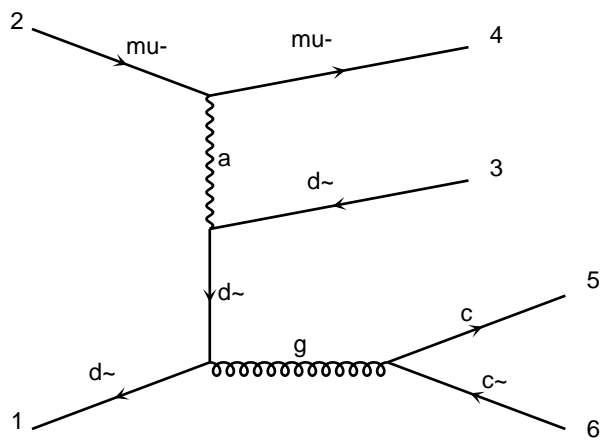

diagram 5

QCD=2, QED=2

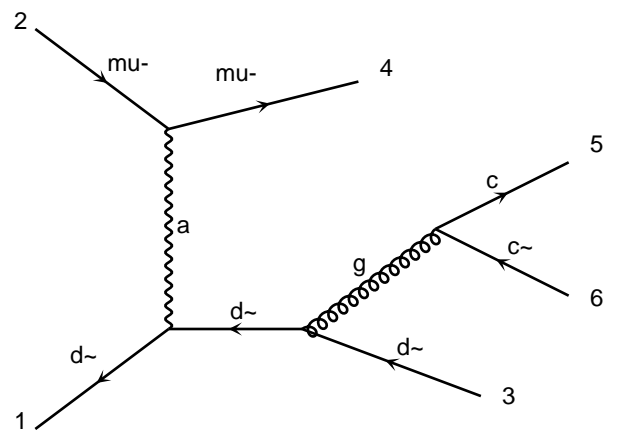

diagram 6

QCD=2, QED=2

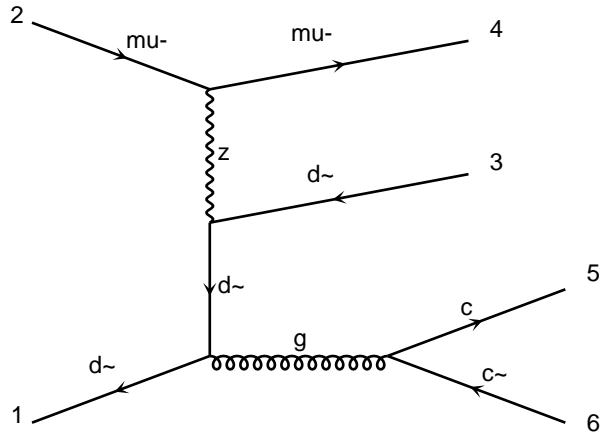

diagram 7

QCD=2, QED=2

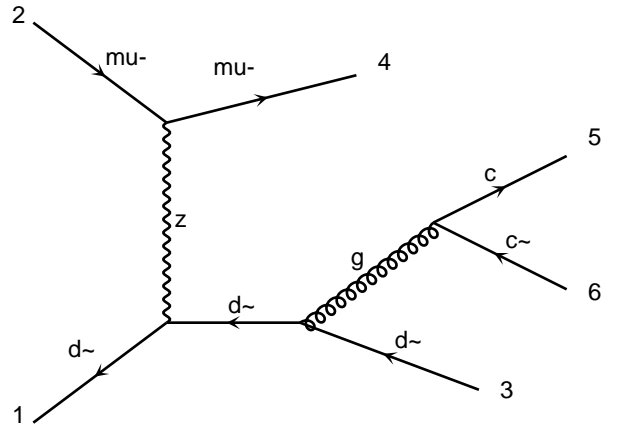

diagram 8

QCD=2, QED=2
