# Supplementary material for: Higgs Production and $H^0 \to c\overline{c}$ at a Future Muon-Ion Collider
Source: arXiv:2211.02615 source file (2022-11-07)
Supplement: Supplementary file 5 [file matrix.pdf]

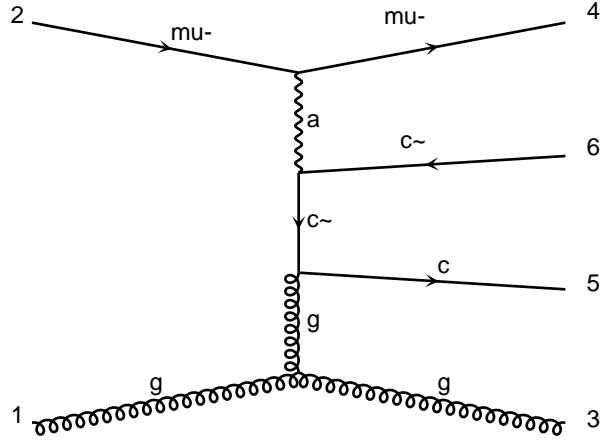

diagram 1 QCD=2, QED=2

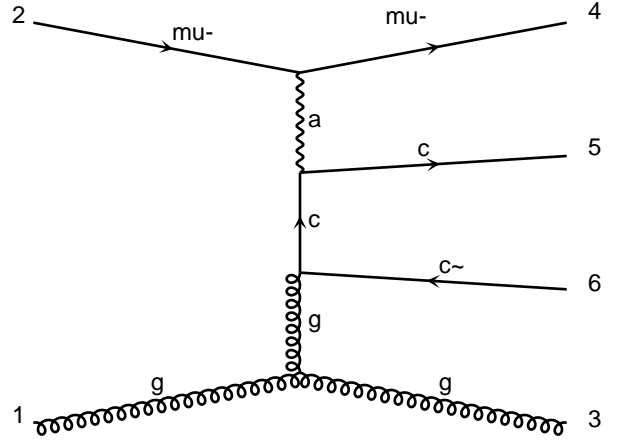

diagram 2 QCD=2, QED=2

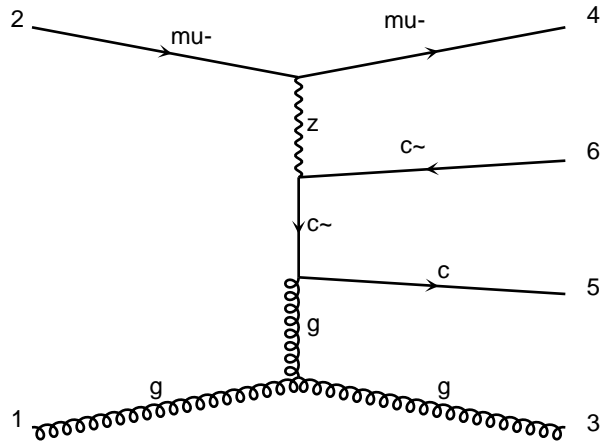

diagram 3 QCD=2, QED=2

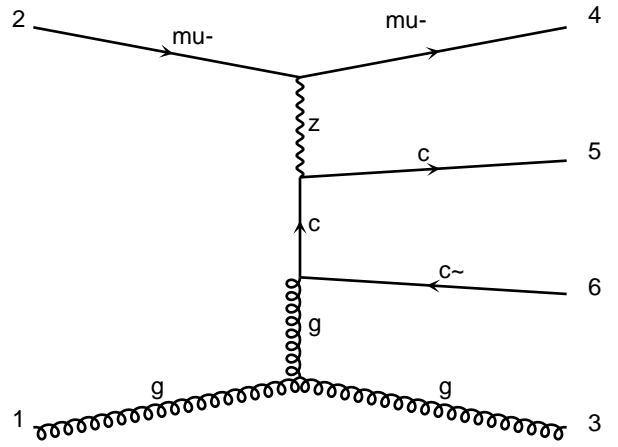

diagram 4 QCD=2, QED=2

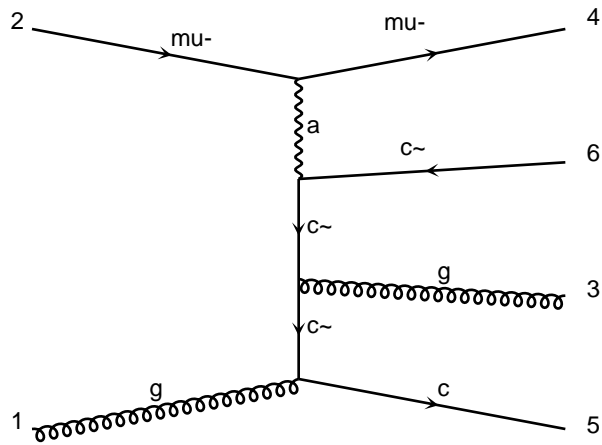

diagram 5 QCD=2, QED=2

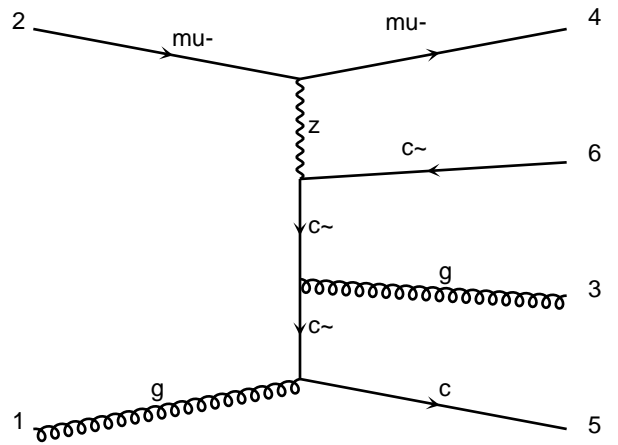

diagram 6 QCD=2, QED=2

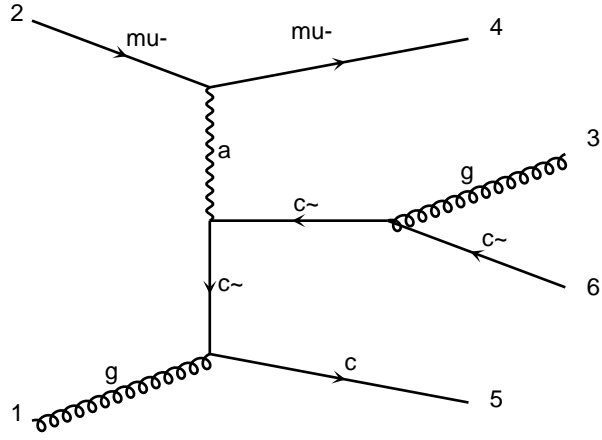

diagram 7

QCD=2, QED=2

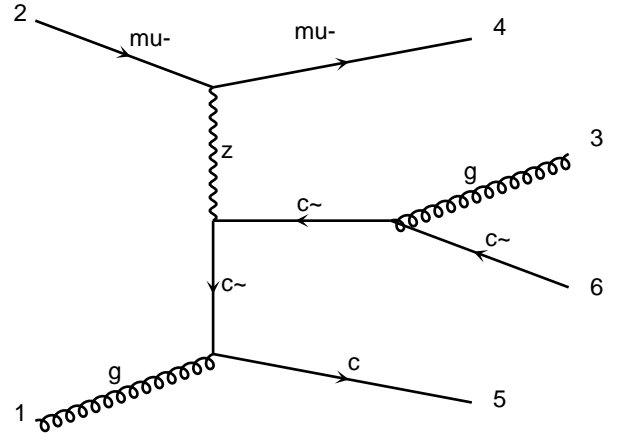

diagram 8

QCD=2, QED=2

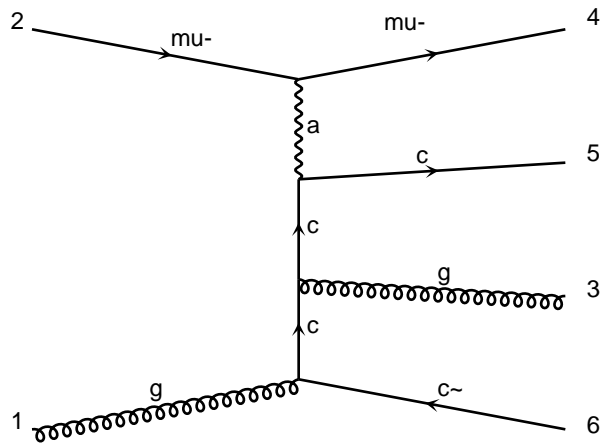

diagram 9

QCD=2, QED=2

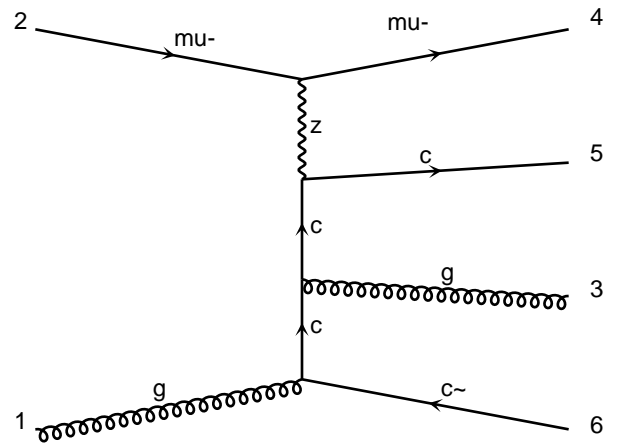

diagram 10

QCD=2, QED=2

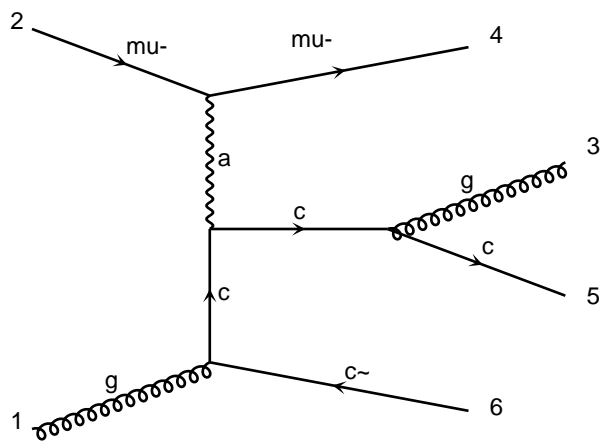

diagram 11

QCD=2, QED=2

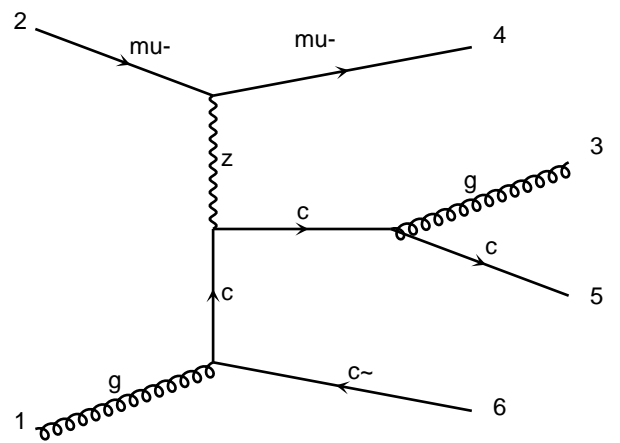

diagram 12

QCD=2, QED=2

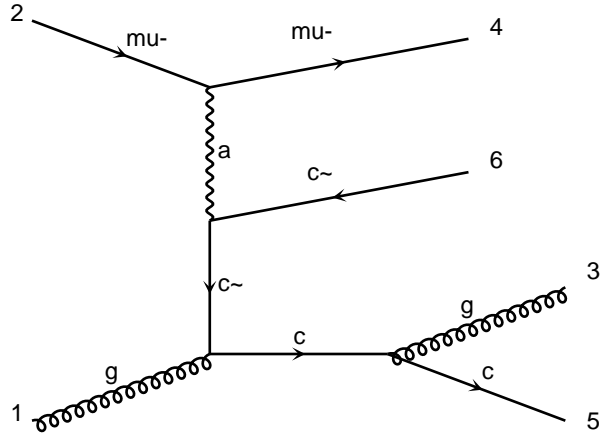

diagram 13      QCD=2, QED=2

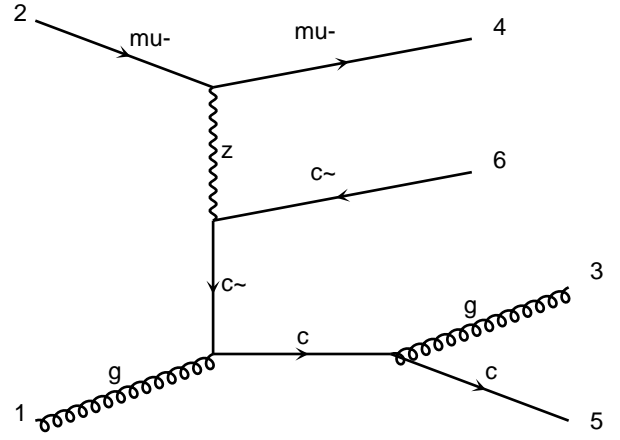

diagram 14      QCD=2, QED=2

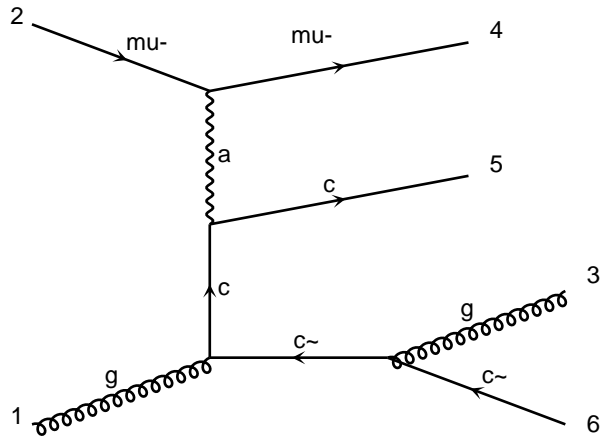

diagram 15      QCD=2, QED=2

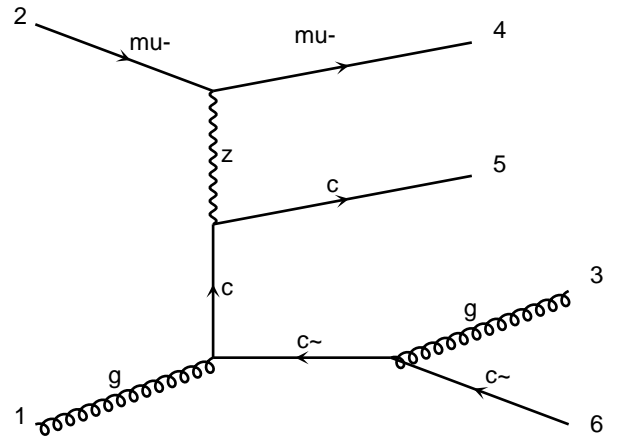

diagram 16      QCD=2, QED=2
